# Supplementary material for: Emergent Fermion Dynamical Symmetry for Monolayer Graphene in a Strong Magnetic Field
Source: arXiv:2312.08475 source file (2023-12-13)
Supplement: Supplementary file 1 [file supplemental.tex]

% This supplement may be run as an include at the end of the main manuscript
% by uncommenting the statement
%
%     \include{supplemental}
%
% at the end of grapheneReview.tex.

\parindent = 12pt

% Zero relevant counters that will be incremented as supplement.tex
% is processed.

\setcounter{page}{1}
\setcounter{equation}{0}

% New counter to keep track of section in Supplement

 \newcounter{suppsectioncounter}
 \setcounter{suppsectioncounter}{0}

% Custom section command for Supplement

\newcommand{\suppsection}[1]{
\setcounter{suppsectioncounter}{\value{suppsectioncounter}+1}
\bigskip\bigskip
\leftline{\large \thesuppsectioncounter.\ \ #1}
\medskip
}

% Make a title page

\thispagestyle{empty}
\widetext    % Set to single column rather than double column

\centerline{\LARGE \textit{Supplement:} Emergent Fermion Dynamical Symmetries for}
\vspace*{3pt}
\centerline{\hfill\LARGE Monolayer Graphene in a Strong Magnetic Field\hfill}

\vspace*{10pt}
\centerline{\large \vphantom{\Huge P} Fletcher Williams, Lianao Wu, and Mike Guidry}

\vspace*{5pt}

\makeNarrowBlurb{
This document provides supplemental material and proofs of some important equations for the review article ``Emergent Fermion Dynamical Symmetries for Monolayer Graphene in a Strong Magnetic Field'' by Mike Guidry, Lianao Wu, and Fletcher Williams, published in the journal {\em Frontiers of Physics} (2024).
}

\suppsection{Introduction}

\noindent
In the following all citations of sections, subsections, equation numbers, figure numbers, and table numbers are by default references to the primary document ``Emergent Dynamical Symmetries for Monolayer Graphene in a Strong Magnetic Field'' published by the present authors in {\em Frontiers of Physics} (2024). If a reference is flagged by ``[this document]'', it is instead a reference to objects in the present Supplement document.

\suppsection{Pairing operators}

\noindent
As a representative example, from \eq{20coupled1.0} the $S=1, M_S = 0, T=0$ 
pair is, 
\begin{equation}
\Adagcoupled{0}{0}{1}{0} =
\sum_{m_k} \sum_{m_1m_2} \sum_{n_1n_2}
\clebsch{\tfrac12}{m_1}{\tfrac12}{m_2}{1}{0}
\clebsch{\tfrac12}{n_1}{\tfrac12}{n_2}{0}{0}
c^\dagger_{m_1 n_1 m_k}
c^\dagger_{m_2 n_2 -m_k}.
\end{equation}
But generally for Clebsch--Gordan coefficients, 
\begin{equation}
    \clebsch{\tfrac12}{n_1}{\tfrac12}{n_2}{0}{0}
    = \frac{(-1)^{1/2-n_1}}{\sqrt2} \,\delta_{n_1, -n_2},
\end{equation}
so that
$$
\Adagcoupled{0}{0}{1}{0} =
\sum_{m_k} \sum_{m_1m_2} \sum_{n_1}
\frac{(-1)^{1/2-n_1}}{\sqrt2}
\clebsch{\tfrac12}{m_1}{\tfrac12}{m_2}{1}{0}
c^\dagger_{m_1 n_1 m_k}
c^\dagger_{m_2 -n_1 -m_k}.
$$
The remaining Clebsch--Gordan coefficient in this expression vanishes unless $m_2 = -m_1$, so
$$
\Adagcoupled{0}{0}{1}{0} =
\sum_{m_k} \sum_{m_1 n_1} 
\frac{(-1)^{1/2-n_1}}{\sqrt2}
\clebsch{\tfrac12}{m_1}{\tfrac12}{-m_1}{1}{0}
c^\dagger_{m_1 n_1 m_k}
c^\dagger_{-m_1 -n_1 -m_k}.
$$
 Writing the four terms in the sum over $m_1$ and $n_1$ out 
explicitly for $n_1 = (-\tfrac12, \tfrac12)$ and $m_1 = (-\tfrac12, 
\tfrac12)$ gives
\begin{align*}
 \Adagcoupled{0}{0}{1}{0} &= -\frac{1}{\sqrt2} \sum_{m_k}
 \clebsch{\tfrac12}{-\tfrac12}{\tfrac12}{\tfrac12}{1}{0}
 c^\dagger_{-\ttfrac12 -\ttfrac12 m_k}
c^\dagger_{\ttfrac12 \ttfrac12  -m_k}
\\
&\quad + \frac{1}{\sqrt2} \sum_{m_k}
 \clebsch{\tfrac12}{-\tfrac12}{\tfrac12}{\tfrac12}{1}{0}
 c^\dagger_{-\ttfrac12 \ttfrac12 m_k}
c^\dagger_{\ttfrac12 -\ttfrac12  -m_k}
\\
&\quad - \frac{1}{\sqrt2} \sum_{m_k}
 \clebsch{\tfrac12}{\tfrac12}{\tfrac12}{-\tfrac12}{1}{0}
 c^\dagger_{\ttfrac12 -\ttfrac12 m_k}
c^\dagger_{-\ttfrac12 \ttfrac12  -m_k}
\\
&\quad + \frac{1}{\sqrt2} \sum_{m_k}
 \clebsch{\tfrac12}{\tfrac12}{\tfrac12}{-\tfrac12}{1}{0}
 c^\dagger_{\ttfrac12 \ttfrac12 m_k}
c^\dagger_{-\ttfrac12 -\ttfrac12  -m_k}.
\end{align*}
Utilizing from \tableref{4.2} [this document] that
$$
\clebsch{\tfrac12}{-\tfrac12}{\tfrac12}{\tfrac12}{1}{0} =
\clebsch{\tfrac12}{\tfrac12}{\tfrac12}{-\tfrac12}{1}{0} = 
\frac{1}{\sqrt2}
$$
we may write
\begin{align}
 \Adagcoupled{0}{0}{1}{0} &= -\frac{1}{2} \sum_{m_k}
 c^\dagger_{-\ttfrac12 -\ttfrac12 m_k}
c^\dagger_{\ttfrac12 \ttfrac12  -m_k}
 + \frac{1}{2} \sum_{m_k}
 c^\dagger_{-\ttfrac12 \ttfrac12 m_k}
c^\dagger_{\ttfrac12 -\ttfrac12  -m_k}
\nonumber
\\
&\quad - \frac{1}{2} \sum_{m_k}
 c^\dagger_{\ttfrac12 -\ttfrac12 m_k}
c^\dagger_{-\ttfrac12 \ttfrac12  -m_k}
+ \frac{1}{2} \sum_{m_k}
 c^\dagger_{\ttfrac12 \ttfrac12 m_k}
c^\dagger_{-\ttfrac12 -\ttfrac12  -m_k}
\nonumber
\\
&=
-\frac{1}{2} \sum_{m_k}
 c^\dagger_{4 m_k}
c^\dagger_{1  -m_k}
 + \frac{1}{2} \sum_{m_k}
 c^\dagger_{2 m_k}
c^\dagger_{3  -m_k}
- \frac{1}{2} \sum_{m_k}
 c^\dagger_{3 m_k}
c^\dagger_{2  -m_k}
+ \frac{1}{2} \sum_{m_k}
 c^\dagger_{1 m_k}
c^\dagger_{4  -m_k}
\nonumber
\\
&=
\frac12 A^\dagger_{14} 
+ \frac12 A^\dagger_{23}
+ \frac12 A^\dagger_{23}
+ \frac12 A^\dagger_{14}
\nonumber
\\
&=
A^\dagger_{14} + A^\dagger_{23},
\end{align}
where in the second equation the mapping between spin and isospin quantum 
numbers and the label $a$ in \fig{grapheneBasis_withTableBW}(a) has been used to 
replace labels $(\sigma,\tau)$ with the label $a$, we have performed 
manipulations such as
$$
-\frac{1}{2} \sum_{m_k}
 c^\dagger_{4 m_k}
c^\dagger_{1  -m_k}
=
\frac{1}{2} \sum_{m_k}
c^\dagger_{1  -m_k}
 c^\dagger_{4 m_k}
 =
\frac{1}{2} \sum_{-m_k}
c^\dagger_{1  m_k}
 c^\dagger_{4 -m_k}
 =\frac12 A^\dagger_{14},
$$
where the first equality is because independent fermion creation operators 
anticommute, the second equality is because $m_k$ is a dummy summation index 
that may be replaced with another summation index, 
and the third equality employed the definition of 
$A^\dagger_{ab}$ in \eq{20algebra1.1}.
The other five possibilities may be determined in a completely analogous way, 
with the results
\begin{equation}
\begin{gathered}
     \Adagcoupled0010 =  
    A_{14}^\dagger + A_{23}^\dagger
    \qquad
    \Adagcoupled1010 = \sqrt 2 \,A_{13}^\dagger
    \qquad
    \Adagcoupled{-1}010 = \sqrt2\, A_{24}^\dagger,
    \\
    \Adagcoupled0001 = A_{14}^\dagger - A_{23}^\dagger
    \qquad
    \Adagcoupled0101 = \sqrt 2\, A_{12}^\dagger
    \qquad
    \Adagcoupled0{-1}01 = \sqrt2\, A_{34}^\dagger.
    \mwgtag{20coupled1.3}
\end{gathered}
\end{equation}
The  hermitian conjugates of these
give the six corresponding 
pair annihilation operators in coupled representation. 
These are the  generators given in \eq{20coupled1.4}, up to a normalization.

To take another example, from \eq{20coupled1.0} the $S=0, T=1, M_T = 1$ 
pair is, 
\begin{equation}
\Adagcoupled{0}{1}{0}{1} =
\sum_{m_k} \sum_{m_1m_2} \sum_{n_1n_2}
\clebsch{\tfrac12}{m_1}{\tfrac12}{m_2}{0}{0}
\clebsch{\tfrac12}{n_1}{\tfrac12}{n_2}{1}{1}
c^\dagger_{m_1 n_1 m_k}
c^\dagger_{m_2 n_2 -m_k}.
\end{equation}
But generally for Clebsch--Gordan coefficients, 
$$
\clebsch{\tfrac12}{m_1}{\tfrac12}{m_2}{0}{0}
= \frac{(-1)^{1/2-m_1}}{\sqrt2} \,\delta_{m_1, -m_2},
$$
so that
$$
\Adagcoupled{0}{1}{0}{1} =
\sum_{m_k} \sum_{n_1n_2} \sum_{m_1}
\frac{(-1)^{1/2-m_1}}{\sqrt2}
\clebsch{\tfrac12}{n_1}{\tfrac12}{n_2}{1}{1}
c^\dagger_{m_1 n_1 m_k}
c^\dagger_{-m_1 n_2 -m_k}.
$$
The remaining Clebsch--Gordan coefficient in this expression vanishes unless $n_1 = n_2 = \frac{1}{2}$, and $\clebsch{\tfrac12}{\tfrac12}{\tfrac12}{\tfrac12}{1}{1} = 1$ so
$$
\Adagcoupled{0}{1}{0}{1} =
\sum_{m_k} \sum_{m_1} 
\frac{(-1)^{1/2-m_1}}{\sqrt2}
c^\dagger_{m_1 \ttfrac12 m_k}
c^\dagger_{-m_1 \ttfrac12 -m_k}.
$$
 Writing the two terms in the sum over $m_1$ out 
explicitly for $m_1 = (-\tfrac12, \tfrac12)$ gives

\begin{align}
 \Adagcoupled{0}{1}{0}{1} &= \frac{1}{\sqrt2} \sum_{m_k}
 c^\dagger_{\ttfrac12 \ttfrac12 m_k}
c^\dagger_{-\ttfrac12 \ttfrac12  -m_k}
 - \frac{1}{\sqrt2} \sum_{m_k}
 c^\dagger_{-\ttfrac12 \ttfrac12 m_k}
c^\dagger_{\ttfrac12 \ttfrac12  -m_k}
\nonumber
\\
&=
\frac{1}{\sqrt2} \sum_{m_k}
 c^\dagger_{1 m_k}
c^\dagger_{2  -m_k}
 - \frac{1}{\sqrt2} \sum_{m_k}
 c^\dagger_{2 m_k}
c^\dagger_{1  -m_k}
\nonumber
\\
&=
\frac{1}{\sqrt2} A^\dagger_{12}
+ \frac{1}{\sqrt2} A^\dagger_{12}
\nonumber
\\
&=
\sqrt2 A^\dagger_{12}.
\end{align}

\suppsection{Coupled representation for particle--hole operators}

\noindent
It is desirable to express the particle--hole generators of \eq{20algebra1.2} in 
coupled representation. Let us begin by introducing a set of operators
\begin{equation}
P_\mu^r = \sum_{m_j m_l} 
(-1)^{{\ttfrac32} + m_\ell}
\clebsch{\tfrac32}{m_j}{\tfrac32}{m_\ell}{
\,r } {\,\mu }
B_{m_j -m_\ell} ,
\mwgtag{multipole1.1}
\end{equation}
with the definition
\begin{equation}
B_{m_j -m_\ell} \equiv \sum_{m_k} c^\dagger_{m_j m_k} 
c^{\vphantom{\dagger}}_{-m_\ell 
m_k}
-\frac14 \delta_{m_j -m_\ell} \Omega,
\mwgtag{multipole1.2}
\end{equation}
where $m_j$ and $m_\ell$ take the values of the fictitious angular 
momentum projection $m_i$ in the table of  \fig{grapheneBasis_withTableBW}(a), providing a 
labeling equivalent to that of $a$ and $b$ in $B_{ab}$, with $m_j$ or $m_\ell$ values 
$\left\{\tfrac32, \tfrac12, -\tfrac12, -\tfrac32 \right\}$
%$\left\{3/2, 1/2, -1/2, -3/2 \right\}$ 
mapping 
to $a$ or $b$ values 
$\left\{ 1,2,3,4\right\}$, respectively.  For example, from  
the table of  \fig{grapheneBasis_withTableBW}(a), 
$
B_{ab} = B_{12}$ and $ B_{m_j m_\ell} = 
B_{\scriptscriptstyle 3/2,1/2}
$
label the same quantity, which is defined in \eq{20algebra1.2}.
From the standard selection rules for coupling of angular momentum, the index $r$ in \eq{multipole1.1} [this document] can take the values $r = 0, 1, 2, 3$, with 
$2r+1$ projections $\mu$ for each possibility, which gives a total of 16 
operators $P^r_\mu$. 
By inserting the explicit values of the Clebsch--Gordan coefficients the  $P_\mu^r$ may be evaluated in terms of the $B_{ab}$.
For example,
 \begin{align*}
 P_0^0 &= \sum_{m_j m_l} 
(-1)^{{\ttfrac32} + m_l}
\clebsch{\tfrac32}{m_j}{\tfrac32}{m_l}{0}{0}
B_{m_j -m_l} 
\\
&=
\frac12 ( B_{-3/2, -3/2} + B_{-1/2, -1/2} + B_{1/2, 1/2} + B_{3/2, 3/2} )
\\
&=
\frac12 ( B_{44} + B_{33} + B_{22} + B_{11} ),
 \end{align*}
 where the mapping between the labels $m_i$ in line 2 and $a$ in line 3 in 
this equation may be found in 
\fig{grapheneBasis_withTableBW}(a), and $B_{ab}$ is defined in 
\eq{20algebra1.2}. 
Evaluating for other values of the indices gives
\begin{equation}
\begin{gathered}
P^0_0 =
 \frac12 (B_{11} + B_{22} + B_{33} + B_{44}) 
=
 \frac12(n_1 + n_2 + n_3 + n_4 -\Omega) =
 \frac12 (n-\Omega),
\\[1pt]
P^1_0 =
 \sqrt{ \frac{9}{20}}(B_{11} - B_{44}) + \sqrt{ \frac{1}{20}}(B_{22} -B_{33})
 % \nonumber
 % \\
 % &
 =
 \sqrt{ \frac{9}{20}}(n_1 - n_4) + \sqrt{ \frac{1}{20}}(n_2 -n_3),
 \\[1pt]
P^1_1 = -\sqrt{ \frac{3}{10}} \,B_{12} - \sqrt{ \frac{4}{10}} \,B_{23}
-\sqrt{ \frac{3}{10}}\, B_{34}
\qquad
 P^1_{-1} =
 \sqrt{ \frac{3}{10}} \,B_{21} + \sqrt{ \frac{4}{10}} \,B_{32}
+\sqrt{ \frac{3}{10}}\, B_{43},
 \\[1pt]
 P^2_0 =
  \frac{1}{2} ( B_{11} - B_{22} + B_{44} - B_{33})
 =  \frac12(n_1 - n_2 + n_4 - n_3)
\qquad
   P^2_1 =
  \frac{1}{\sqrt{2}} (B_{34} - B_{12}),
\\[1pt]
 P^2_{-1} =  \frac{1}{\sqrt2} (B_{21} - B_{43})
\qquad
 P^2_2  =
 - \frac{1}{\sqrt{2}} (B_{13} + B_{24})
 \qquad
 P^2_{-2} =
 - \frac{1}{\sqrt2} (B_{31} + B_{42}),
 \\[1pt]
  P^3_0  =
 \sqrt{ \frac{1}{20}} (B_{11} - B_{44}) 
 + \sqrt{ \frac{9}{20}} (B_{33}-B_{22})
  =
 \sqrt{ \frac{1}{20}} (n_1 - n_4) 
 - \sqrt{ \frac{9}{20}} (n_2 - n_3),
 \\[1pt]
  P^3_1  =
-\sqrt{ \frac15} B_{12} + \sqrt{ \frac35} B_{23} - \sqrt{ \frac15} B_{34}
\qquad
 P^3_{-1}  =
 \sqrt{ \frac15} B_{21} - \sqrt{ \frac35} B_{32}
 + \sqrt{ \frac15} B_{43},
 \\[1pt]
  P^3_2  =
 \sqrt{ \frac12} (B_{24} -  B_{13})
 \qquad
  P^3_{-2}=
 \sqrt{ \frac12} (B_{42} - B_{31})
\qquad
 P^3_3  =
 -B_{14}
 \qquad
 P^3_{-3} =
 B_{41}.
\end{gathered}
 \mwgtag{PofB}
\end{equation}
where the quantities $n_i$ given by
\begin{equation}
n_i = B_{ii} = \sum_{m_k} c^\dagger_{im_k} c_{im_k} - \frac14 \Omega
\mwgtag{numberOperators}
\end{equation}
are number operators for each of the four states and
the total particle number $n$ is the sum over the four states labeled by
$a$ in  the table of  \fig{grapheneBasis_withTableBW}(a),
$
 n = n_1 + n_2 + n_3 + n_4 = {\rm total\ particle\ number} .
$
It will be convenient  to sometimes replace the operator $P_0^0$ 
with the operator $S_0$, according to 
\begin{equation}
S_0 \equiv \frac12 (n-\Omega) = P^0_0,
 \mwgtag{p0n}
\end{equation}
where  $2\Omega$ is 
the degeneracy of 
the space for the particles that participate in the SO(8) symmetry.
Physically $S_0 = \tfrac12 (n-\Omega)$ is one half 
the particle number measured from half filling (which corresponds to 
$n=\Omega$).

\suppsection{Transformations between different basis states}

\noindent
In exploring dynamical symmetries of the \SO8 algebra 
\eqnoeq{20algebraTotal} it is often useful to use different basis sets for the generators. 
This section gathers the relationships between the different sets of basis vectors employed in the main text. For brevity in the following,
$
\{P^1, P^2, P^3, S_0, S, S^\dagger, D\phantomdagger_{\mu}, 
D^\dagger_\mu \}
$
will be termed  the nuclear \SO8 basis and 
$
\{ \spin_\alpha,  \,T_\alpha,\, N_\alpha, \,\Piop \alpha x, \,
\Piop \alpha y,  S_0, S, 
S^\dagger, D\phantomdagger_{\mu}, D^\dagger_\mu \}
$
will be termed the graphene \SO8 basis.

First note that the \SO8 particle--hole operators 
\eqnoeq{20algebra1.2} can be replaced by the operators of \eq{20algebra1.4} 
through a comparison of their definitions.  For example, consider the spin 
operator $\spin_y$.  From \eq{20algebra1.4},
\begin{align*}
\spin_y &=
 \sum_{m_k}
\sum_{ \tau \sigma \sigma'} \mel{\sigma'}{\sigma_y}{\sigma}
c^\dagger_{\tau\sigma'm_k} c_{\tau\sigma m_k\vphantom{'}}\phd
\\
&=
\sum_{m_k}
\left(
-i c^\dagger_{+\uparrow m_k} c_{+\downarrow m_k\vphantom{\downarrow}}\phd
+ i c^\dagger_{+\downarrow m_k} c_{+\uparrow m_k\vphantom{\downarrow}}\phd 
-i c^\dagger_{-\uparrow m_k} c_{-\downarrow 
m_k\vphantom{\downarrow}}\phd
+ i c^\dagger_{-\downarrow m_k} c_{-\uparrow m_k\vphantom{\downarrow}}\phd
\right)
\\
&= -iB_{12} + i B_{21} -i B_{34} +i B_{43},
\end{align*}
where the standard $2\times2$ Pauli matrix representation for $\sigma_2 = 
\sigma_y$ was employed and equivalences between the indices $a$ and 
$(\tau,\sigma)$ in the table of \fig{grapheneBasis_withTableBW}(a) were used to 
map to   indices for $B_{ab}$. The results for the complete set of operators are displayed in Eqs.\ \eqnoeq{algebra1.8}-\eqnoeq{algebra1.11}.

In transforming from the nuclear SO(8) basis to the graphene SO(8) basis  
the particle number (charge) operator $n$ or $S_0$ and the 12 pairing operators 
$\{D_\mu, \, D^\dagger_\mu,\, S,\, S^\dagger\}$ are retained, but 
the 15 SU(4) 
generators $\{ P^1,\, P^2, \,P^3\}$ in the nuclear representation are 
replaced with the 15 
SU(4) generators $\{\spin_\alpha,\,  T_\alpha,\, N_\alpha, \,\Piop \alpha x, 
\,\Piop \alpha y\}$ defined in the graphene representation of \eq{20algebra1.4}.
The explicit transformation from the  $\{ P^1,\, P^2,\, P^3\}$ generators to the 
$\{\spin_\alpha,  \,T_\alpha,\, N_\alpha, \,\Piop \alpha x, \, \Piop \alpha y\}$ 
generators is given by
\begin{gather}
\spin_x =
\sqrt{\frac{6}{5}}\left(P^1_{-1} - P^1_1 \right) + 
\frac{2}{\sqrt5}\left(P^3_{-1} - P^3_1 \right)
% \mwgtag{ngx1}
% \\
\nonumber
\qquad
\spin_y =
i\left[\sqrt{\frac{6}{5}}\left(P^1_1 + P^1_{-1}\right) + 
\frac{2}{\sqrt5}\left(P^3_1 + P^3_{-1}\right)\right],
%\mwgtag{ngx2}
\nonumber
\\
\spin_z =
\frac{2}{\sqrt5} P^1_0 + \frac{4}{\sqrt5} P_0^3 = n_1 -n_2 + n_3 -n_4
% \mwgtag{ngx3}
% \\
\qquad
T_x =
-\sqrt2 \left( P^2_2 + P^2_{-2}\right)
% \mwgtag{ngx4}
% \\
\qquad
T_y =
i\sqrt2 \left( P^2_2 - P^2_{-2}\right),
\nonumber
%\mwgtag{ngx5}
\\
T_z =
\frac{4}{\sqrt 5} P^1_0 - \frac{2}{\sqrt5} P^3_0 = n_1 + n_2 -n_3 -n_4
\mwgtag{ngx6}
\qquad
N_x =
\frac{1}{\sqrt2}\left(P^2_{-1} - P^2_1\right)
% \mwgtag{ngx7}
% \\
\qquad
N_y =
\frac{i}{\sqrt2}\left(P^2_{-1} + P^2_1\right),
%\mwgtag{ngx8}
\nonumber
\\
N_z =
P^2_0 = n_1 - n_2 + n_4 - n_3
\qquad
\Piop xx =
\frac{1}{2}\left[ \vphantom{\sqrt{\frac{2}{5}}} P^3_{-3} - P^3_3 
+\sqrt{\frac{2}{5}}\left(P^1_{-1} - 
P^1_1\right)  + \sqrt{\frac{3}{5}}\left(P^3_1 - P^3_{-1}\right)\right],
\mwgtag{ngx}
\\
\Piop yx =
\frac{i}{2}\left[ \sqrt{\frac{2}{5}} P^3_{-3} + P^3_3 
+ \sqrt{\frac{2}{5}}\left(P^1_{-1} + 
P^1_1\right)  - \sqrt{\frac{3}{5}}\left(P^3_1 + P^3_{-1}\right)\right]
\qquad
\Piop zx =
-\frac{1}{\sqrt2} \left( P^3_2 + P^3_{-2}\right),
\nonumber
\\
\Piop xy =
\frac{i}{2}\left[\sqrt{\frac{2}{5}} P^3_{-3} + P^3_3 
- \sqrt{\frac{2}{5}}\left(P^1_{-1} + 
P^1_1\right) + \sqrt{\frac{3}{5}}\left(P^3_1 + P^3_{-1}\right)\right]
\qquad
\Piop zy =
-\frac{i}{\sqrt2} \left( P^3_2 - P^3_{-2}\right),
\nonumber
\\
\Piop yy =
\frac{1}{2}\left[ \vphantom{\sqrt{\frac{2}{5}}} -P^3_{-3} + P^3_3 
- 
\sqrt{\frac{2}{5}}\left(P^1_1 - P^1_{-1}\right) + 
\sqrt{\frac{3}{5}}\left(P^3_1 - P^3_{-1}\right)\right] .
\nonumber
\end{gather}
In Eqs.\ \eqnoeq{algebra1.8}--\eqnoeq{algebra1.11} (and in Eqs.\ \ref{eq:ngx} [this document]) the graphene 
basis $\{\spin_\alpha,\,  T_\alpha,\, N_\alpha, \,\Piop \alpha x, \,\Piop \alpha 
y\}$ has been expressed in terms of the generators $B_{ab}$ defined in 
\eq{20algebra1.2}.  The 
inverse transformations giving the $B_{ab}$ generators in terms of the $\{\spin_\alpha,\,  
T_\alpha,\, N_\alpha, \,\Piop \alpha x, \,\Piop \alpha y\}$ generators are
\cite{wu2017}
\begin{equation}
\begin{gathered}
B_{12} =
\frac{1}{2}N_{x}+\frac{1}{2}iN_{y}+\frac{1}{4}\spin_{x}+\frac{1}{4}i\spin_{y}
\qquad
B_{13} =
\frac{1}{4}T_{x}+\frac{1}{4}iT_{y}+\frac{1}{2}\Pi_{zx}-\frac{1}{2}i\Pi_{zy},
%mwgtag{grapheneToB2}
\\
B_{14} =
\frac{1}{2}\Pi _{xx}-\frac{1}{2}i\,\Pi _{yx}-\frac{1}{2}i\Pi _{xy}-
\frac{1}{2}\Pi _{yy}
\qquad
B_{23} =
\frac{1}{2}\Pi _{xx}+\frac{1}{2}i\,\Pi _{yx}-\frac{1}{2}i\,\Pi _{xy}+
\frac{1}{2}\Pi _{yy},
\\
B_{24} =
\frac{1}{4}T_{x}+\frac{1}{4}i\,T_{y}-\frac{1}{2}\Pi _{zx}+\frac{1}{2}
i\,\Pi _{zy}
\qquad
B_{34} =
\frac{1}{4}\spin_{x}-\frac{1}{2}i\,N_{y}-\frac{1}{2}N_{x}+\frac{1}{4}i\,\spin_{y},
\\
B_{11} =
\frac14\spin_z +\frac14 T_z + \frac12 N_z + \frac14 (n-\Omega)
\qquad
B_{22} =
-\frac14\spin_z +\frac14 T_z - \frac12 N_z + \frac14 (n-\Omega),
\\
B_{33} =
\frac14\spin_z -\frac14 T_z - \frac12 N_z + \frac14 (n-\Omega)
\qquad
B_{44} =
-\frac14\spin_z -\frac14 T_z + \frac12 N_z + \frac14 (n-\Omega),
%mwgtag{grapheneToB10}
\end{gathered}
\mwgtag{grapheneToB}%
\end{equation}
where the unlisted operators may be obtained from $B_{ba} = B_{ab}^\dagger$
and the diagonal operators have been assumed to obey the \unitary4 constraint
\begin{equation}
 B_{11} + B_{22} + B_{33} + B_{44} =   n-\Omega,
 \mwgtag{u4Constraint}
\end{equation}
with $n = n_1 + n_2 + n_3 + n_4$ the total particle number and $\Omega$ the 
total pair degeneracy given by \eq{20degen1.2}.

\suppsection{Lie algebra in the nuclear SO(8) basis}

\noindent
Because the six operators defined by \eq{20coupled1.4}, their six hermitian 
conjugates, and the 16 operators defined by \eq{multipole1.1}  [this document] are independent 
linear combinations of the SO(8) generators defined in Eqs.\ \eqnoeq{20algebra1.1} 
and \eqnoeq{20algebra1.2}, the 28 operators $\{P^\ell_\mu,\, S, \, S^\dagger, \, D_\mu, \,
D^\dagger_\mu\}$ also close an SO(8) algebra under commutation. 
The 
SO(8) commutation relations for the coupled-representation generators 
$$
G^{\,\prime}_{\scriptscriptstyle{\rm SO(8)}}=\{ P^1,\, P^2,\, P^3, 
    \,
    S_0, \,
    S, \,S^\dagger, \,D\phantomdagger_{\mu},\, D^\dagger_\mu \}
    $$ 
 in \eq{20nuclearBasis} are given explicitly by 
\cite{gin80,wu1994}
\begin{subequations}
\begin{align}
 \comm{S}{S^\dagger} &=
 -2S_0 ,
 \mwgtag{commcoupled1.1}
 \\
 \comm{D_{\mu'}}{D^\dagger_{\mu}} &=
 -2\delta_{\mu\mu'} S_0 + \sum_{t {\rm\ odd}} (-1)^{\mu'}
 \clebsch{2,}{-\mu'}{2}{\mu}{\,t,}{\mu-\mu'}
 \sixj{2}{2}{t}{\frac32}{\frac32}{\frac32}
 P_{\mu,-\mu'}^t ,
\mwgtag{commcoupled1.2}
\\
\comm{D_\mu^\dagger}{S} &= P_\mu^2,
\mwgtag{commcoupled1.3}
\\
\comm{P^r_\mu}{S^\dagger} &=
2 \delta_{r2}D^\dagger_\mu + 2 \delta_{r0} \delta_{\mu0} S^\dagger,
\mwgtag{commcoupled1.4}
\\
\comm{P_{\mu'}^r}{D_\mu^\dagger} &=
2(-1)^{\mu'} \delta_{r2} \delta_{-\mu\mu'}
-4\sqrt{5(2r+1)}
% \nonumber
% \\
% &\qquad\times\ 
\clebsch{r}{\mu'}{2}{\mu}{2,}{\mu+\mu'}
\sixj{2}{2}{r}{\frac32}{\frac32}{\frac32}
D_{\mu+\mu'}^\dagger ,
\mwgtag{commcoupled1.5}
\\
\comm{P^r_{\mu'}}{P^s_\mu} &=
2 (-1)^{r+s} \sqrt{(2r+1)(2s+1)} 
\,\,\sum_t 
\clebsch{r}{{\mu'}}{s}{{\mu}}{\,t,}{{
\mu+\mu'} }
% \nonumber
% \\
% &\quad
%\times 
\left[1-(-1)^{r+s+t}\right]
\sixj{r}{s}{t}{\frac32}{\frac32}{\frac32}
P^{\,t}_{\mu+\mu'} ,
\mwgtag{commcoupled1.6}
\end{align}
 \mwgtag{commcoupled}%
 \end{subequations}
where $S_0$ is defined in \eq{p0n} and $\{\,\}$ denotes the Wigner 6-$j$ symbol \cite{des74} for the recoupling of three angular momenta to good total angular 
momentum.

 \suppsection{Tables\label{clebsch-3j}}

\noindent
For convenience we include below Table \ref{tb:4.2} [this document] of Clebsch--Gordan coefficients and Table \ref{tb:4.1} [this document] of $3J$-symbols, with the Clebsch--Gordan coefficients $\cg$ and $3J$-symbols related by
    \begin{equation}
       \threej {j_1}{j_2}{J}{m_1}{m_2}{-M}=
       \frac{\phase {j_1-j_2+M}}{\sqrt{2J+1}} \cg .
       \mwgtag {4.66}
   \end{equation}
The values of these vector coupling coefficients are useful in various proofs contained in this Supplement. 

%  Arguments in makerowl and makerowr: j1,j2,m1,m2,J,M,Clebsch
%  Use together  to make row of table
\newcommand{\makerowl}[7]{$#1$&$#2$&$#3$&$#4$&$#5$&$#6$&$#7$&}
\newcommand{\makerowr}[7]{$\qquad#1$&$#2$&$#3$&$#4$&$#5$&$#6$&$#7$}

\begin{table}
%\begin{adjustwidth}{-\extralength}{0cm} % Make table wide

%\centering
\caption{Some \SO3 Clebsch--Gordan Coefficients
$\left<j_1m_1j_2m_2 | JM \right>$ from Ref.\ \cite{guid2022}\protect\label{tb:4.2}}
\begin{small}
\setlength{\tabcolsep}{4 pt}
\begin{tabular}{|c|c|c|c|c|c|c||c|c|c|c|c|c|c|}
\hline
$j_1$ &  $j_2$ & $m_1$ & $m_2$ & $J$ & $M$ & CG &
$\qquad j_1$ &  $j_2$ & $m_1$ & $m_2$ & $J$ & $M$ & CG    
\\
\hline
\makerowl {1/2}{1/2}{1/2}{1/2}111
\makerowr {1/2}{1/2}{1/2}{-1/2}10{\sqrt{1/2}}
\\
\makerowl {1/2}{1/2}{1/2}{-1/2}00{\sqrt{1/2}}
\makerowr {1/2}{1/2}{-1/2}{1/2}10{\sqrt{1/2}}
\\
\makerowl {1/2}{1/2}{-1/2}{1/2}00{-\sqrt{1/2}}
\makerowr {1/2}{1/2}{-1/2}{-1/2}{1}{-1}1
\\
\hline
\makerowl 1{1/2}1{1/2}{3/2}{3/2}{1}
\makerowr 1{1/2}1{-1/2}{3/2}{1/2}{\sqrt{1/3}}
\\
\makerowl 1{1/2}1{-1/2}{1/2}{1/2}{\sqrt{2/3}}
\makerowr 1{1/2}0{1/2}{3/2}{1/2}{\sqrt{2/3}}
\\
\makerowl 1{1/2}0{1/2}{1/2}{1/2}{-\sqrt{1/3}}
\makerowr 1{1/2}0{-1/2}{3/2}{-1/2}{\sqrt{2/3}}
\\
\makerowl 1{1/2}0{-1/2}{1/2}{-1/2}{\sqrt{1/3}}
\makerowr 1{1/2}{-1}{1/2}{3/2}{-1/2}{\sqrt{1/3}}
\\
\makerowl 1{1/2}{-1}{1/2}{1/2}{-1/2}{-\sqrt{2/3}}
\makerowr 1{1/2}{-1}{-1/2}{3/2}{-3/2}{1}
\\
\hline 
\makerowl 1111221
\makerowr 111021{\sqrt{1/2}}
\\
\makerowl 111011{\sqrt{1/2}}
\makerowr 110121{\sqrt{1/2}}
\\
\makerowl 110111{-\sqrt{1/2}}
\makerowr 111{-1}20{\sqrt{1/6}}
\\
\makerowl 111{-1}10{\sqrt{1/2}}
\makerowr 111{-1}00{\sqrt{1/3}}
\\
\makerowl 110020{\sqrt{2/3}}
\makerowr 1100100
\\
\makerowl 110000{-\sqrt{1/3}}
\makerowr 11{-1}120{\sqrt{1/6}}
\\
\makerowl 11{-1}110{-\sqrt{1/2}}
\makerowr 11{-1}100{\sqrt{1/3}}
\\
\makerowl 110{-1}2{-1}{\sqrt{1/2}}
\makerowr 110{-1}1{-1}{\sqrt{1/2}}
\\
\makerowl 11{-1}02{-1}{\sqrt{1/2}}
\makerowr 11{-1}01{-1}{-\sqrt{1/2}}
\\
\makerowl 11{-1}{-1}2{-2}1
\makerowr {}{}{}{}{}{}{}{}
\\
\hline
\makerowl 2{1/2}2{1/2}{5/2}{5/2}1
\makerowr 2{1/2}1{-1/2}{5/2}{3/2}{\sqrt{1/5}}
\\
\makerowl 2{1/2}2{-1/2}{3/2}{3/2}{\sqrt{4/5}}
\makerowr 2{1/2}1{1/2}{5/2}{3/2}{\sqrt{4/5}}
\\
\makerowl 2{1/2}1{1/2}{3/2}{3/2}{-\sqrt{1/5}}
\makerowr 2{1/2}1{-1/2}{5/2}{1/2}{\sqrt{2/5}}
\\
\makerowl 2{1/2}1{-1/2}{3/2}{1/2}{\sqrt{3/5}}
\makerowr 2{1/2}0{1/2}{5/2}{1/2}{\sqrt{3/5}}
\\
\makerowl 2{1/2}0{1/2}{3/2}{1/2}{-\sqrt{2/5}}
\makerowr 2{1/2}0{-1/2}{5/2}{-1/2}{\sqrt{3/5}}
\\
\makerowl 2{1/2}0{-1/2}{3/2}{-1/2}{\sqrt{2/5}}
\makerowr 2{1/2}{-1}{1/2}{5/2}{-1/2}{\sqrt{2/5}}
\\
\makerowl 2{1/2}{-1}{1/2}{3/2}{-1/2}{-\sqrt{3/5}}
\makerowr 2{1/2}{-1}{-1/2}{5/2}{-3/2}{\sqrt{4/5}}
\\
\makerowl 2{1/2}{-1}{-1/2}{3/2}{-3/2}{\sqrt{1/5}}
\makerowr 2{1/2}{-2}{1/2}{5/2}{-3/2}{\sqrt{1/5}}
\\
\makerowl 2{1/2}{-2}{1/2}{3/2}{-3/2}{-\sqrt{4/5}}
\makerowr 2{1/2}{-2}{-1/2}{5/2}{-5/2}1
\\
\hline
\makerowl {3/2}{1/2}{3/2}{1/2}221
\makerowr {3/2}{1/2}{3/2}{-1/2}21{1/2}
\\
\makerowl {3/2}{1/2}{3/2}{-1/2}11{\sqrt{3/4}}
\makerowr {3/2}{1/2}{1/2}{1/2}21{\sqrt{3/4}}
\\
\makerowl {3/2}{1/2}{1/2}{1/2}11{-1/2}
\makerowr {3/2}{1/2}{1/2}{-1/2}20{\sqrt{1/2}}
\\
\makerowl {3/2}{1/2}{1/2}{-1/2}10{\sqrt{1/2}}
\makerowr {3/2}{1/2}{-1/2}{1/2}20{\sqrt{1/2}}
\\
\makerowl {3/2}{1/2}{-1/2}{1/2}10{-\sqrt{1/2}}
\makerowr {3/2}{1/2}{-1/2}{-1/2}2{-1}{\sqrt{3/4}}
\\
\makerowl {3/2}{1/2}{-1/2}{-1/2}1{-1}{1/2}
\makerowr {3/2}{1/2}{-3/2}{1/2}{2}{-1}{1/2}
\\
\makerowl {3/2}{1/2}{-3/2}{1/2}{1}{-1}{-\sqrt{3/4}}
\makerowr {3/2}{1/2}{-3/2}{-1/2}2{-2}1
\\
\hline
\end{tabular}
\end{small}
%\end{adjustwidth}
\end{table}

\newlength{\tspace}
\setlength{\tspace}{11pt}
\newcommand{\symtwo}{b}

\begin{table}
%\begin{adjustwidth}{-\extralength}{0cm} % Make table wide
%\centering
\caption{Some $3J$ coefficients $\threej {j_1}{j_2}{J}{m_1}{m_2}{M}$
from Ref.\ \reference{bri68}
\label{tb:4.1}}
\setlength{\tabcolsep}{0pt}
\begin{tabular}{l}
%\begin{eqnarray*}
$\threeJ{a}{a+1/2}{1/2}{\symtwo  }{-\symtwo   -1/2}{1/2}
=(-1)^{a-\symtwo  -1}\left[\dfrac
{a+\symtwo  +1}
{(2a+1)(2a+2)}
\right]^{1/2}$
\\[\tspace]
$\threeJ{a}{a}{1}{\symtwo  }{-\symtwo   -1}{1}
=(-1)^{a-\symtwo  }\left[\dfrac
{(a-\symtwo  )(a+\symtwo  +1)}
{2a(a+1)(2a+1)}
\right]^{1/2}$
\\[\tspace]
$\threeJ{a}{a}{1}{\symtwo  }{-\symtwo  }{0}
=(-1)^{a-\symtwo  }\dfrac
{\symtwo  }
{[a(a+1)(2a+1)]^{1/2}}
$
\\[\tspace]
$\threeJ{a}{a+1}{1}{\symtwo  }{-\symtwo   -1}{1}
=(-1)^{a-\symtwo  }\left[\dfrac
{(a+\symtwo  +1)(a+\symtwo  +2)}
{(2a+1)(2a+2)(2a+3)}
\right]^{1/2}$
\\[\tspace]
$\threeJ{a}{a+1}{1}{\symtwo  }{-\symtwo  }{0}
=(-1)^{a-\symtwo  -1}\left[\dfrac
{(a-\symtwo  +1)(a+\symtwo  +1)}
{(a+1)(2a+1)(2a+3)}
\right]^{1/2}$
\\[\tspace]
$\threeJ{a}{a+1/2}{3/2}{\symtwo  }{-\symtwo   -3/2}{3/2}
=(-1)^{a-\symtwo  -1}\left[\dfrac
{3(a+\symtwo  +1)(a+\symtwo  +2)(a-\symtwo  )}
{2a(2a+1)(2a+2)(2a+3)}
\right]^{1/2}$
\\[\tspace]
$\threeJ{a}{a+1/2}{3/2}{\symtwo  }{-\symtwo   -1/2}{1/2}
=(-1)^{a-\symtwo  } (a-3\symtwo  )\left[\dfrac
{a+\symtwo  +1}
{2a(2a+1)(2a+2)(2a+3)}
\right]^{1/2}$
\\[\tspace]
$\threeJ{a}{a+3/2}{3/2}{\symtwo  }{-\symtwo   -3/2}{3/2}
=(-1)^{a-\symtwo  -1} \left[\dfrac
{(a+\symtwo   +1)(a+\symtwo   +2)(a+\symtwo  +3)}
{(2a+1)(2a+2)(2a+3)(2a+4)}
\right]^{1/2}$
\\[\tspace]
$\threeJ{a}{a+3/2}{3/2}{\symtwo  }{-\symtwo   -1/2}{1/2}
=(-1)^{a-\symtwo  } \left[\dfrac
{3(a-\symtwo   +1)(a+\symtwo   +1)(a+\symtwo  +2)}
{(2a+1)(2a+2)(2a+3)(2a+4)}
\right]^{1/2}$
\\[\tspace]
$\threeJ{a}{a}{2}{\symtwo  }{-\symtwo   -2}{2}
=(-1)^{a-\symtwo  } \left[\dfrac
{3(a+\symtwo   +1)(a+\symtwo   +2)(a-\symtwo  -1)(a-\symtwo  )}
{a(2a+3)(2a+2)(2a+1)(2a-1)}
\right]^{1/2}$
\\[\tspace]
$\threeJ{a}{a}{2}{\symtwo  }{-\symtwo   -1}{1}
=(-1)^{a-\symtwo  } (2\symtwo  +1) \left[\dfrac
{3(a-\symtwo  )(a+\symtwo  +1)}
{a(2a+3)(2a+2)(2a+1)(2a-1)}
\right]^{1/2}$
\\[\tspace]
$\threeJ{a}{a}{2}{\symtwo  }{-\symtwo  }{0}
=(-1)^{a-\symtwo  } \dfrac
{3\symtwo  ^2-a(a+1)}
{[a(a+1)(2a+3)(2a+1)(2a-1)]^{1/2}}
$
\\[\tspace]
$\threeJ{a}{a+1}{2}{\symtwo  }{-\symtwo  -2}{2}
=(-1)^{a-\symtwo  }\left[\dfrac
{(a+\symtwo  +1)(a+\symtwo  +2)(a+\symtwo   +3)(a-\symtwo  )}
{a(a+1)(2a+4)(2a+3)(2a+1)}
\right]^{1/2}$
\\[\tspace]
$\threeJ{a}{a+1}{2}{\symtwo  }{-\symtwo  -1}{1}
=(-1)^{a-\symtwo  -1} (a-2\symtwo  ) \left[\dfrac
{(a+\symtwo  +2)(a+\symtwo  +1)}
{a(a+1)(2a+4)(2a+3)(2a+1)}
\right]^{1/2}$
\\[\tspace]
$\threeJ{a}{a+1}{2}{\symtwo  }{-\symtwo  }{0}
=(-1)^{a-\symtwo  -1} \symtwo   \left[\dfrac
{3(a+\symtwo  +1)(a-\symtwo  +1)}
{a(a+1)(a+2)(2a+3)(2a+1)}
\right]^{1/2}$
\\[\tspace]
$\threeJ{a}{a+2}{2}{\symtwo  }{-\symtwo  -2}{2}
=(-1)^{a-\symtwo  }\left[\dfrac
{(a+\symtwo  +1)(a+\symtwo  +2)(a+\symtwo  +3)(a+\symtwo  +4)}
{(2a+1)(2a+2)(2a+3)(2a+4)(2a+5)}
\right]^{1/2}$
\\[\tspace]
$\threeJ{a}{a+2}{2}{\symtwo  }{-\symtwo  -1}{1}
=(-1)^{a-\symtwo -1 }\left[\dfrac
{(a+\symtwo  +1)(a+\symtwo  +2)(a+\symtwo  +3)(a-\symtwo  +1)}
{(a+1)(a+2)(2a+1)(2a+3)(2a+5)}
\right]^{1/2}$
\\[\tspace]
$\threeJ{a}{a+2}{2}{\symtwo  }{-\symtwo  }{0}
=(-1)^{a-\symtwo  }\left[\dfrac
{3(a+\symtwo  +1)(a+\symtwo  +2)(a-\symtwo  +1)(a-\symtwo  +2)}
{(a+1)(2a+5)(2a+4)(2a+3)(2a+1)}
\right]^{1/2}$
%\end{eqnarray*}
\end{tabular}
%\end{adjustwidth}
\end{table}

%\end{supple}
